# Supplementary material for: Weakly Supervised Video Individual CountingWeakly Supervised Video Individual Counting
Source: arXiv:2312.05923 source file (2023-12-10)
Supplement: Supplementary file 1 [file 7_appendix.tex]

\clearpage
\setcounter{page}{1}
\maketitlesupplementary

\section{More about UAVVIC}
\begin{table}[t]
    \centering
   \resizebox{\linewidth}{!}{
   \begin{tabular}{c| c| c |c |c}
    \hline
    \multirow{2}{*}{Methods} & \multirow{2}{*}{Stationary} & Up and & Horizontally & \multirow{2}{*}{Rotating} \\
        & & down & moving & \\
        \toprule
    Bot-Sort~\cite{botsort}& 40.1& 47.5& 59.7 & 62.1\\
    Deep-OC-Sort~\cite{deepocsort}& 35.8 & 36.9& 42.2&42.1 \\
    DRNet~\cite{DRVIC} & 13.9 & 15.4& 24.4 & 25.1\\\hline
    CGNet& ~~9.7& 12.0& 13.2& 14.6\\\hline
    \end{tabular}}
    \caption{Results in terms of MAE under different kinds of camera settings. 
    % with Bot-Sort~\cite{botsort}, Deep-OC-Sort~\cite{deepocsort}, DRNet~\cite{DRVIC}, and our CGNet. 
    }
    \label{tab:camera}
\end{table}

\begin{figure}
    \centering
    \begin{subfigure}{.45\linewidth}
        \includegraphics[width=\linewidth]{figs/uavvic_attr_pie.png}
        \caption{}
    \end{subfigure}\hfill
    \begin{subfigure}{.45\linewidth}
        \includegraphics[width=\linewidth]{figs/uavvic_attr_bar.png}
        \caption{}
    \end{subfigure}
    \caption{(a) The ratio of different UAV (camera) movements in our UAVVIC. (b) The average inflow and outflow per frame in UAVVIC over different UAV (camera) movements.}
    \label{fig:cameradist}
\end{figure}

\begin{figure}[!htp]
    \centering
    \begin{subfigure}{\linewidth}
        \centering
        \includegraphics[width=.31\linewidth]{figs/0001.jpg}
        \includegraphics[width=.31\linewidth]{figs/0002.jpg}
        \includegraphics[width=.31\linewidth]{figs/0003.jpg}
        \caption{Stationary camera}
    \end{subfigure}
    \begin{subfigure}{\linewidth}
        \centering
        \includegraphics[width=.31\linewidth]{figs/5828.jpg}
        \includegraphics[width=.31\linewidth]{figs/5848.jpg}
        \includegraphics[width=.31\linewidth]{figs/5850.jpg}
        \caption{Up and down moving camera}
    \end{subfigure}
        \begin{subfigure}{\linewidth}
        \centering
        \includegraphics[width=.31\linewidth]{figs/1572.jpg}
        \includegraphics[width=.31\linewidth]{figs/1573.jpg}
        \includegraphics[width=.31\linewidth]{figs/1574.jpg}
        \caption{Horizontally moving camera}
    \end{subfigure}
    \begin{subfigure}{\linewidth}
        \centering
        \includegraphics[width=.31\linewidth]{figs/1532.jpg}
        \includegraphics[width=.31\linewidth]{figs/1536.jpg}
        \includegraphics[width=.31\linewidth]{figs/1545.jpg}
        \caption{Rotating camera}
    \end{subfigure}
    \caption{Different camera movements in our UAVVIC dataset.}
    \label{fig:camera}
\end{figure}

\begin{figure*}[htp]
    \centering

        \begin{subfigure}{.32\textwidth}
        \centering
        \includegraphics[width=\linewidth]{figs/uavvic/6465.jpg}
        \caption{0s}
    \end{subfigure}\hfill
    \begin{subfigure}{.32\textwidth}
        \centering
        \includegraphics[width=\linewidth]{figs/uavvic/6466.jpg}
        \caption{3s}
    \end{subfigure}\hfill
    \begin{subfigure}{.32\textwidth}
        \centering
        \includegraphics[width=\linewidth]{figs/uavvic/6467.jpg}
        \caption{6s}
    \end{subfigure}
    
    \begin{subfigure}{.32\textwidth}
        \centering
        \includegraphics[width=\linewidth]{figs/uavvic/6490.jpg}
        \caption{21s}
    \end{subfigure}\hfill
    \begin{subfigure}{.32\textwidth}
        \centering
        \includegraphics[width=\linewidth]{figs/uavvic/6491.jpg}
        \caption{24s}
    \end{subfigure}\hfill
    \begin{subfigure}{.32\textwidth}
        \centering
        \includegraphics[width=\linewidth]{figs/uavvic/6492.jpg}
        \caption{27s}
    \end{subfigure}
    
    \begin{subfigure}{.32\textwidth}
        \centering
        \includegraphics[width=\linewidth]{figs/uavvic/7308.jpg}
        \caption{90s}
    \end{subfigure}\hfill
    \begin{subfigure}{.32\textwidth}
        \centering
        \includegraphics[width=\linewidth]{figs/uavvic/7309.jpg}
        \caption{93s}
    \end{subfigure}\hfill
    \begin{subfigure}{.32\textwidth}
        \centering
        \includegraphics[width=\linewidth]{figs/uavvic/7310.jpg}
        \caption{96s}
    \end{subfigure}
    
    \begin{subfigure}{.32\textwidth}
        \centering
        \includegraphics[width=\linewidth]{figs/uavvic/7315.jpg}
        \caption{99s}
    \end{subfigure}\hfill
    \begin{subfigure}{.32\textwidth}
        \centering
        \includegraphics[width=\linewidth]{figs/uavvic/7316.jpg}
        \caption{102s}
    \end{subfigure}\hfill
    \centering
    \begin{subfigure}{.32\textwidth}
        \centering
        \includegraphics[width=\linewidth]{figs/uavvic/7317.jpg}
        \caption{105s}
    \end{subfigure}
    
    \begin{subfigure}{.32\textwidth}
        \centering
        \includegraphics[width=\linewidth]{figs/uavvic/7318.jpg}
        \caption{108s}
    \end{subfigure}\hfill
    \begin{subfigure}{.32\textwidth}
        \centering
        \includegraphics[width=\linewidth]{figs/uavvic/7319.jpg}
        \caption{111s}
    \end{subfigure}\hfill
    \begin{subfigure}{.32\textwidth}
        \centering
        \includegraphics[width=\linewidth]{figs/uavvic/7320.jpg}
        \caption{114s}
    \end{subfigure}

    \begin{subfigure}{.32\textwidth}
        \centering
        \includegraphics[width=\linewidth]{figs/uavvic/7321.jpg}
        \caption{117s}
    \end{subfigure}\hfill
    \begin{subfigure}{.32\textwidth}
        \centering
        \includegraphics[width=\linewidth]{figs/uavvic/7322.jpg}
        \caption{120s}
    \end{subfigure}\hfill
    \begin{subfigure}{.32\textwidth}
        \centering
        \includegraphics[width=\linewidth]{figs/uavvic/7323.jpg}
        \caption{123s}
    \end{subfigure}
    
    \caption{Result visualization of our CGNet on a video in our UAVVIC dataset with horizontally moving camera. Pink, blue, yellow, and green dots denote pedestrians, cars, buses, and vans, respectively. Red dots denote the predicted inflows.}
    \label{fig:visuavvic1}
\end{figure*}

The video length in our UAVVIC dataset is longer than that of existing VIC datasets. Specifically, the average, maximum, and minimum video length on UAVVIC is about 75, 315, and 18 seconds, while the average, maximum, and minimum video length on SenseCrowd is about 20, 44, and 4 seconds. 
%The proposed UAVVIC dataset contains 221 videos with an average/max/min length of 75s/315s/18s, which is longer than another big dataset, SenseCrowd~\cite{sensecrowd}, the average/max/min length of which is 20s/44s/4s. 
The average number of pedestrians, cars, buses, and vans in each frame is 50, 23, 4, and 1, respectively. The density of pedestrians is larger than that in SenseCrowd, which is 37. The average inflow per frame in the UAVVIC dataset is 6.6, larger than that in SenseCrowd, which is 4.1. This is caused by the camera movement in the UAVVIC dataset, resulting in more inflows.

%To better evaluate the performance of our method on different ,we manually annotate the 634 videos
We manually annotate the types of UAV or camera movement for comprehensive evaluation. The movement of the UAV (camera) is classified into four categories: stationary, up and down, horizontal moving, and rotation.  Fig.~\ref{fig:camera} shows images captured in these four scenarios. 
%As shown in Fig.~\ref{fig:camera}, the camera movement categories in this data set include a fixed camera, up and down moving camera, a horizontally moving camera, and a rotating camera, and 
As shown in Fig.~\ref{fig:cameradist}(a), the number of videos for these four categories is 75, 11, 75, and 60, respectively.  The performance of CGNet and existing methods~\cite{botsort,deepocsort,DRVIC} on each movement category is shown in \cref{tab:camera}. 
%A moving camera makes it hard for the VIC task as it challenges models to handle the re-entering problems. 
As shown in Fig.~\ref{fig:cameradist}(b), the inflow and outflow in videos shot by moving cameras are much larger, making it more difficult to count individuals. Therefore, all methods have a performance drop on moving cameras, especially on the horizontally moving and rotating cameras, as shown in \cref{tab:camera}. %The average inflow and outflow per frame over different movement categories are shown in Fig.~\ref{fig:cameradist}. 
A visualization result for a video with camera movement type horizontal moving is shown in Fig.~\ref{fig:visuavvic1}. 

\begin{figure*}[!hbt]
\begin{subfigure}{\textwidth}
\centering
\includegraphics[width=0.92\linewidth]{figs/q3.png}
\caption{Previous frame~(0s)}
\end{subfigure}

\begin{subfigure}{\textwidth}
\centering
\includegraphics[width=0.92\linewidth]{figs/q4.png}
\caption{Current frame~(3s)}
\end{subfigure}

\begin{subfigure}{\textwidth}
\centering
\includegraphics[width=0.92\linewidth]{figs/q7.png}
\caption{Previous frame~(0s)}
\end{subfigure}

\begin{subfigure}{\textwidth}
\centering
\includegraphics[width=0.92\linewidth]{figs/q8.png}
\caption{Current frame~(3s)}
\end{subfigure}

\begin{subfigure}{\textwidth}
\centering
\includegraphics[width=0.92\linewidth]{figs/q9.png}
\caption{Previous frame~(0s)}
\end{subfigure}

\begin{subfigure}{\textwidth}
\centering
\includegraphics[width=0.92\linewidth]{figs/q10.png}
\caption{Current frame~(3s)}
\end{subfigure}
\caption{Results on the SenseCrowd dataset. Red dots are predictions of the locator. Blue/green/yellow circles are correct predicted inflow, error predicted inflow, and missed inflow, respectively. }
\label{fig:quality}
\end{figure*}

\section{Performance with Individual-level Association Label}
\begin{table}[]
    \centering
    \begin{tabular}{c|c c c c}
         \hline
         Ratio& MAE & MSE & WRAE  \\\hline
         0\% & 8.86 & 17.69 & 9.27\\ 
         25\% & 8.64 & 16.5 & 8.71\\
         50\% & 8.30 & 15.72 & 8.69\\
         100\%& 8.12 & 15.57 & 8.39\\
         \hline
    \end{tabular}
    \caption{Performance of our CGNet with different ratios of individual-level association annotations.}
    \label{tab:sup}
\end{table}
Our method can work easily with supervised annotations. Given individual-level associations, the latent variable $\Omega$ can be replaced, and thus $\mathcal{L}_{scon}$ can be calculated directly. As shown in \cref{tab:sup}, with the help of individual-level association annotations, the performance of CGNet is further improved. Although more individual-level association labels are helpful for CGNet, the improvement is not significant. For example, using all the individual-level annotations only reduces the MAE by 0.74 (8.12 VS 8.86), demonstrating that an exact individual-level association label may not be necessary for VIC.

\section{Qualitative Results on SenseCrowd}
We provide more visualization results in \cref{fig:quality}.
